# Supplementary material for: The hybrid radio/X-ray correlation of the black hole transient MAXI J1348-630
Source: arXiv:2105.06006 ancillary file (2021-05-13)
Supplement: Supplementary file 1 [file Supplementary_material.pdf]

# MN-21-1190-L – Supplementary material

Table 1: Radio flux densities and unabsorbed X-ray fluxes selected for the radio/X-ray correlation presented in this work, along with the radio spectral index (when available) and the telescopes used for obtaining the data (see Carotenuto et al. 2021). Upper limits are reported at the $3\sigma$ level.

| MJD | Outburst phase | X-ray flux[b] 1–10 keV | Radio flux density [mJy] | Spectral index[c] $\alpha$ | Telescopes |
|---|---|---|---|---|---|
| 58509.9 | Main outburst – rise | $38.1 \pm 0.3$ | $3.4 \pm 0.1$ | $0.02 \pm 0.09$ | ATCA/*Swift* |
| 58511.0 | – | $201 \pm 20$ | $6.2 \pm 0.4$ | $0.1 \pm 0.2$ | ATCA/*Swift*[a] |
| 58512.0 | – | $346 \pm 35$ | $13.70 \pm 0.05$ | | MeerKAT/*Swift*[a] |
| 58514.0 | – | $528 \pm 53$ | $21.9 \pm 0.8$ | $0.18 \pm 0.02$ | ATCA/*Swift*[a] |
| 58515.2 | – | $590 \pm 59$ | $28.6 \pm 0.1$ | | MeerKAT/*Swift*[a] |
| 58515.9 | – | $625 \pm 3$ | $34.4 \pm 1.4$ | | ATCA/*Swift* |
| 58519.9 | – | $1320 \pm 132$ | $135 \pm 1$ | $0.155 \pm 0.003$ | ATCA/*Swift*[a] |
| 58602.1 | Main outburst – decay | $113 \pm 11$ | $4.73 \pm 0.04$ | | MeerKAT/*Swift*[a] |
| 58603.3 | – | $89 \pm 9$ | $8.7 \pm 0.1$ | $0.09 \pm 0.05$ | ATCA/*Swift*[a] |
| 58607.9 | – | $32 \pm 3$ | $3.43 \pm 0.04$ | | MeerKAT/*Swift*[a] |
| 58608.7 | – | $26 \pm 3$ | $2.75 \pm 0.06$ | | ATCA/*Swift*[a] |
| 58612.4 | – | $9.1 \pm 0.3$ | $0.77 \pm 0.02$ | $0.21 \pm 0.02$ | ATCA/*Swift* |
| 58614.9 | – | $4.2 \pm 0.4$ | $0.32 \pm 0.04$ | | MeerKAT/*Swift*[a] |
| 58617.5 | – | $2.0 \pm 0.2$ | $0.71 \pm 0.02$ | $0.27 \pm 0.03$ | ATCA/*Swift*[a] |
| 58621.9 | – | $0.52 \pm 0.05$ | $0.27 \pm 0.04$ | | MeerKAT/*Swift*[a] |
| 58628.0 | First reflare – rise | $0.047 \pm 0.005$ | $0.13 \pm 0.04$ | | MeerKAT/*Swift*[a] |
| 58629.3 | – | $0.15 \pm 0.02$ | $0.15 \pm 0.01$ | $0.0 \pm 0.2$ | ATCA/*Swift*[a] |
| 58634.9 | – | $8.7 \pm 0.9$ | $0.79 \pm 0.06$ | | MeerKAT/*Swift*[a] |
| 58642.9 | – | $67 \pm 7$ | $4.34 \pm 0.06$ | | MeerKAT/*Swift*[a] |
| 58643.5 | – | $74 \pm 7$ | $4.09 \pm 0.02$ | $-0.03 \pm 0.02$ | ATCA/*Swift*[a] |
| 58650.9 | – | $99 \pm 2$ | $6.26 \pm 0.09$ | | MeerKAT/*Swift* |
| 58658.8 | – | $103 \pm 10$ | $4.60 \pm 0.05$ | | MeerKAT/*Swift*[a] |
| 58660.3 | First reflare – decay | $102 \pm 10$ | $4.18 \pm 0.04$ | $0.05 \pm 0.03$ | ATCA/*Swift*[a] |
| 58664.7 | – | $69 \pm 7$ | $3.86 \pm 0.05$ | | MeerKAT/*Swift*[a] |
| 58671.9 | – | $54 \pm 5$ | $2.29 \pm 0.03$ | | MeerKAT/*Swift*[a] |
| 58678.9 | – | $43 \pm 4$ | $1.66 \pm 0.03$ | | MeerKAT/*Swift*[a] |
| 58686.9 | – | $24 \pm 2$ | $1.11 \pm 0.03$ | | MeerKAT/*Swift*[a] |
| 58689.4 | – | $19.3 \pm 0.4$ | $1.19 \pm 0.01$ | $-0.02 \pm 0.03$ | ATCA/*Swift* |
| 58691.8 | – | $11 \pm 1$ | $0.70 \pm 0.03$ | | MeerKAT/*Swift*[a] |
| 58699.7 | – | $0.98 \pm 0.05$ | $0.44 \pm 0.04$ | | MeerKAT/*Swift* |
| 58705.8 | – | $0.071 \pm 0.007$ | $0.14 \pm 0.04$ | | MeerKAT/*Swift* |
| 58726.7 | – | $<0.002$ | $<0.12$ | | MeerKAT/*Swift*[a] |
| 58727.1 | – | $<0.005$ | $<0.033$ | | ATCA/*Swift*[a] |
| 58775.6 | Second reflare – decay | $0.008 \pm 0.004$ | $<0.12$ | | MeerKAT/*Swift* |
| 58782.6 | – | $<0.01$ | $<0.12$ | | MeerKAT/*Swift*[a] |
| 58789.6 | – | $<0.006$ | $<0.06$ | | ATCA/*Swift*[a] |
| 58817.4 | Third reflare – decay | $0.67 \pm 0.07$ | $0.47 \pm 0.03$ | | MeerKAT/*Swift*[a] |
| 58820.7 | – | $0.21 \pm 0.02$ | $0.56 \pm 0.01$ | $0.19 \pm 0.06$ | ATCA/*Swift*[a] |
| 58824.4 | – | $0.059 \pm 0.006$ | $0.16 \pm 0.03$ | | MeerKAT/*Swift*[a] |
| 58827.8 | – | $0.016 \pm 0.002$ | $0.15 \pm 0.01$ | $0.9 \pm 0.2$ | ATCA/*Swift*[a] |
| 58831.3 | – | $0.002 \pm 0.001$ | $0.054 \pm 0.006$ | $-0.3 \pm 0.3$ | ATCA/*Swift* |
| 58894.1 | Fourth reflare – decay | $0.21 \pm 0.02$ | $0.22 \pm 0.02$ | | MeerKAT/*Swift*[a] |
| 59112.7 | Seventh reflare – decay | $0.08 \pm 0.02$ | $0.17 \pm 0.02$ | | MeerKAT/*Swift* |
| 59127.0 | – | 0.003[d] $\pm$ 0.001 | $0.09 \pm 0.01$ | $-1.2 \pm 0.3$ | ATCA/*Swift*[d] |

[a] Interpolated X-ray flux.

[b] In units of $10^{-10}$ erg cm$^{-2}$ s$^{-1}$.

[c] Only computed for ATCA multi-frequency observations. For the results reported in the Discussion, we also added values of $\alpha$ reported in Carotenuto et al. (2021) for detections of compact jets at epochs for which we did not have a corresponding X-ray observation: $\alpha = 0.31 \pm 0.04$ (MJD 58814) and $\alpha = 0.4 \pm 0.3$ (MJD 58830).

[d] The corresponding X-ray flux was extrapolated (and not interpolated) from the *Swift*/XRT light curve, as the last X-ray observation of our monitoring was performed $\sim$36 h before the radio observation. We add a conservative 30% error to this measurement.

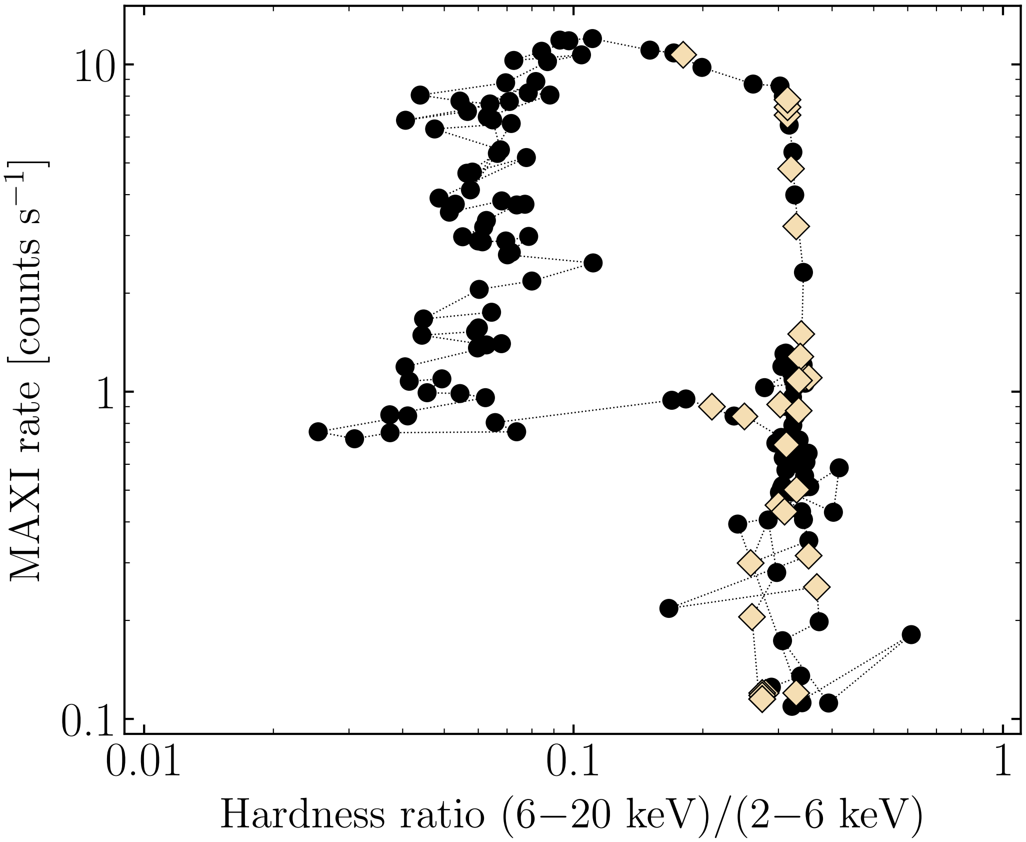


Figure 1: Hardness-intensity diagram (HID) of MAXI J1348–630 during its main outburst, where the hardness ratio (HR) was determined from MAXI data. For clarity, we only show MAXI observations in the MJD interval 58505–58710 with a count rate above 0.1 counts s$^{-1}$, thus including the brightest part of the outburst, which tracked an entire cycle in the HID. The beige diamonds mark the time of radio observations used for the radio/X-ray correlation on the HID. Radio observations taken during the second part of the outburst (MJD > 58710) lie on the bottom part of the hard-line ($0.3 \lesssim$ HR $\lesssim 0.4$).
